# Supplementary material for: OV-DINO: Unified Open-Vocabulary Detection with Language-Aware Selective Fusion
Source: arXiv:2407.07844 source file (2024-07-22)
Supplement: Supplementary file 1 [file 12_appendix.tex]

{\appendices
\section*{Proof of the First Zonklar Equation}
Appendix one text goes here.
You can choose not to have a title for an appendix if you want by leaving the argument blank
\section*{Proof of the Second Zonklar Equation}
Appendix two text goes here.}
